# Supplementary material for: Online Trajectory Replanner for Dynamically Grasping Irregular Objects
Source: arXiv:2501.17968 source file (2025-01-29)
Supplement: Supplementary file 1 [file appendix.tex]

\label{section: Limits}
\begin{table}[htbp]
	\begin{center}%[table-unit-alignment=left]	
		\begin{tabular}{lc}
			\hline
			Param. & Value \\
			\hline
			$\underline{\vec{q}_\mathrm{G}}$ & [\SI{0}{\milli\meter}; \SI{-10}{\degree}; \SI{-30}{\milli\meter}; \SI{160}{\milli\meter}] \\
			$\overline{\vec{q}_\mathrm{G}}$ & [\SI{80}{\milli\meter}; \SI{10}{\degree}; \SI{30}{\milli\meter}; \SI{170}{\milli\meter}] \\
			$\underline{\vec{q}_\hsym}$ & [\SI{-90}{\degree}; \SI{-90}{\degree}; \SI{-90}{\degree}; \SI{-90}{\degree}] \\
			$\overline{\vec{q}_\hsym}$ & [\SI{90}{\degree}; \SI{90}{\degree};\SI{90}{\degree}; \SI{90}{\degree}] \\			
			$\underline{\dot{\vec{q}}_\hsym}$ & [\SI{-100}{\degree\per\second}; \SI{-100}{\degree\per\second}; \SI{-100}{\degree\per\second}; \SI{-100}{\degree\per\second}] \\
			$\overline{\dot{\vec{q}}_\hsym}$ & [\SI{100}{\degree\per\second}; \SI{100}{\degree\per\second}; \SI{100}{\degree\per\second}; \SI{100}{\degree\per\second}] \\
			$\underline{\ddot{\vec{q}}_\hsym}$ & 1000$\cdot$[\SI{-0,4}{\degree\per\second\squared}; \SI{-1,5}{\degree\per\second\squared};\SI{-0,4}{\degree\per\second\squared}; \SI{-1,5}{\degree\per\second\squared}] \\
			$\overline{\ddot{\vec{q}}_\hsym}$ & 1000$\cdot$[\SI{0,4}{\degree\per\second\squared}; \SI{1,5}{\degree\per\second\squared}; \SI{0,4}{\degree\per\second\squared}; \SI{1,5}{\degree\per\second\squared}] \\				
			$\underline{\Delta \vec{p}_0^\hsym}$ & [\SI{-0,5}{mm}; \SI{-0,5}{mm}; \SI{-0,5}{mm}] \\
			$\overline{\Delta \vec{p}_0^\hsym}$ & [\SI{0,5}{mm}; \SI{0,5}{mm}; \SI{0,5}{mm}] \\
			\hline
		\end{tabular}
	\end{center}
	\caption{Limitations of the gripper state $\mathbf{q}_\hsym$ and the grasping state $\mathbf{q}_\mathrm{G}$.}
	\label{tab:limits}
\end{table}
